# Supplementary material for: High-Performance Thermoelectric Oxides Based on Spinel Structure
Source: arXiv:2008.09759 ancillary file (2020-08-22)
Supplement: Supplementary file 1 [file supplement2.pdf]

# Supporting Information
# High-Performance Thermoelectric Oxides Based on Spinel Structure

M. Hussein N. Assadi*
*School of Materials Science and Engineering, UNSW Sydney, NSW, 2052, Australia.*

J. Julio Gutiérrez Moreno
*Institute for Advanced Study, Shenzhen University, Shenzhen 518060, China, and*
*Key Laboratory of Optoelectronic Devices and Systems of Ministry of Education and Guangdong Province,*
*College of Physics and Optoelectronic Engineering, Shenzhen University, Shenzhen 518060, China.*

Marco Fronzi
*School of Mathematical and Physical Science, University of Technology Sydney, Sydney, NSW 2007, Australia.*
(Dated: 2020)

## SUPPLEMENTARY FIGURES

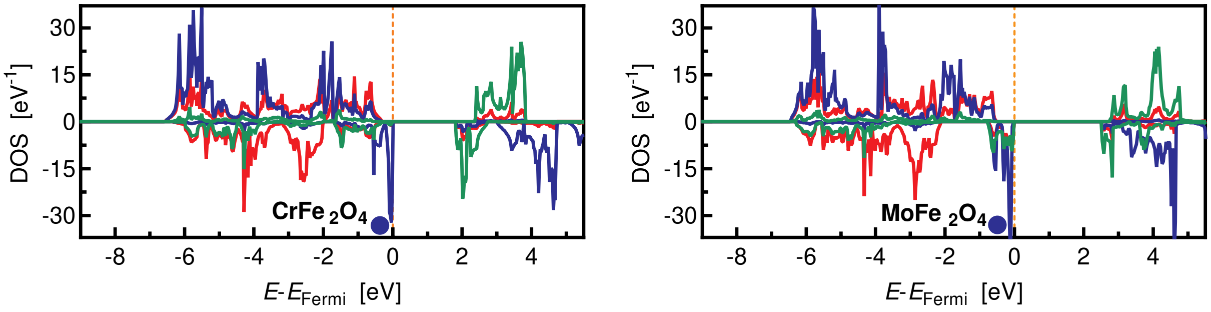


Figure S1. PDOS of the best performing compounds, $CrFe_2O_4$ on the left and $MoFe_2O_4$ on the right, calculated with larger $U$ and $J$ values. The values used here were $U(\mathrm{Fe}) = 5.8$ eV, $J(\mathrm{Fe}) = 0.5$ eV, $U(\mathrm{Cr}) = 4.2$ eV, $J(\mathrm{Cr}) = 0.5$ eV, $U(\mathrm{Mo}) = 4.9$ eV, $J(\mathrm{Mo}) = 0.5$ eV. These values are commonly used for similar oxides archived in Materials Project (`https://materialsproject.org`). The blue, green, and red lines denote Fe 3d, TM d, and O 2p states. The blue dots show the strong localization of the Fe 3d states just below the Fermi level, similar to the DOS presented in **Figure 2** and **Figure 3**. The band gaps are, however, slightly wider when compared to the DOS reported in **Figure 2(b)** and **Figure 3(b)**.

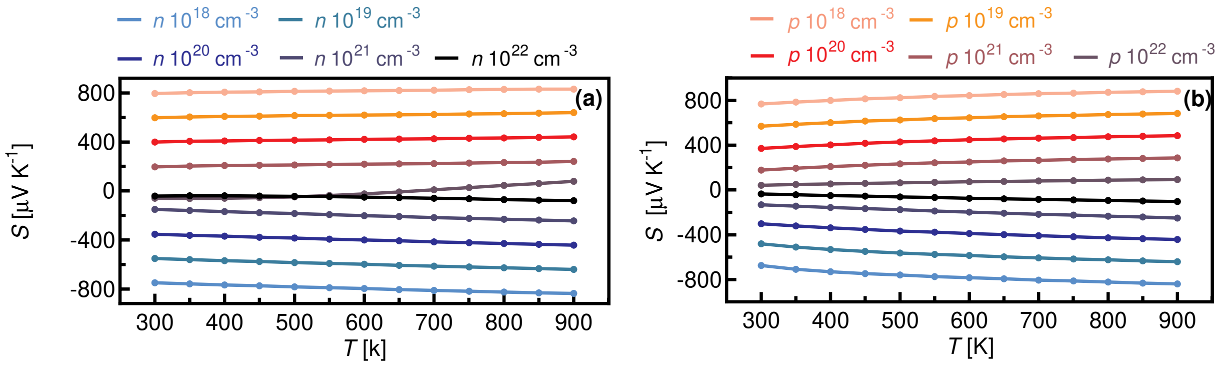


Figure S2. The Seebeck coefficient ($S$) for the best-performing compounds (a) $CrFe_2O_4$ and (b) $MoFe_2O_4$ as a function of temperature for various doping levels calculated with alternative $U$ and $J$ values of Figure S1. The values here are slightly higher than the ones reported in **Figure 4(b)** and **Figure 5(b)**. One can, therefore, assumes the values presented in **Figure 4** and **Figure 5** were conservative.

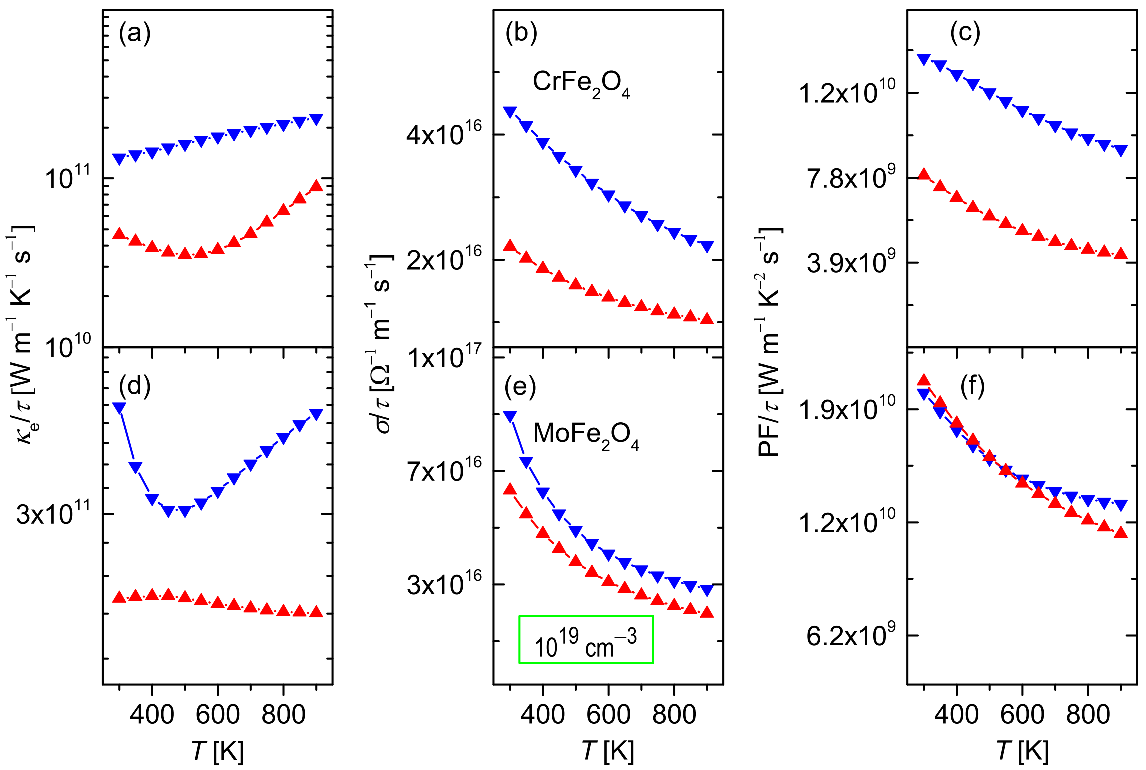


Figure S3. Thermoelectric characteristics of the best-performing compounds at a doping level of $10^{19}$ carriers/cm$^3$ calculated with alternative $U$ and $J$ values of Figure S1. $\tau$, $\kappa_e$, $\sigma$, and PF stand for relaxation time, electronic contribution to the thermal conductivity, electric conductivity, and power factor, respectively. Red and blue symbols indicate hole and electron doping, respectively. $\kappa_e\,/\,\tau$ values (a, d) obtained here are generally lower, while PF/$\tau$ values (c, f) are generally higher than the values presented in **Figure 6**. $\sigma\,/\,\tau$ (b, e), however, is not significantly affected.

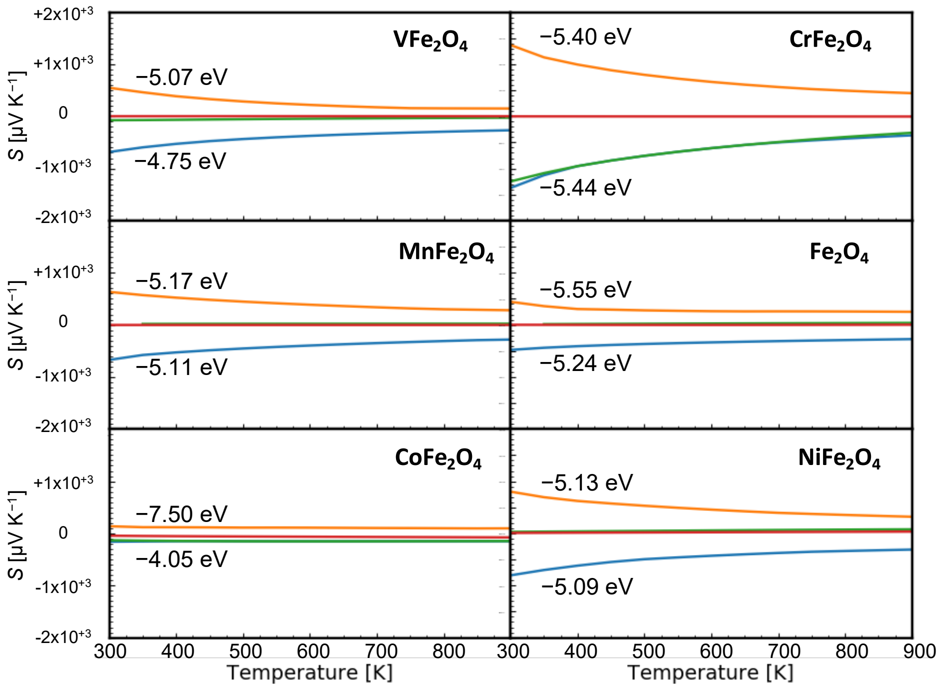


Figure S4. The Seebeck coefficient ($S$) for the 3d TM containing $TMFe_2O_4$ compounds as a function of temperature at different chemical potentials. The blue and orange lines indicate the chemical potentials for which $S$ was an absolute extreme. The values reported here for extreme $S$ are, however, only hypothetical as the required shifts in chemical potentials cannot be easily achieved with doping.

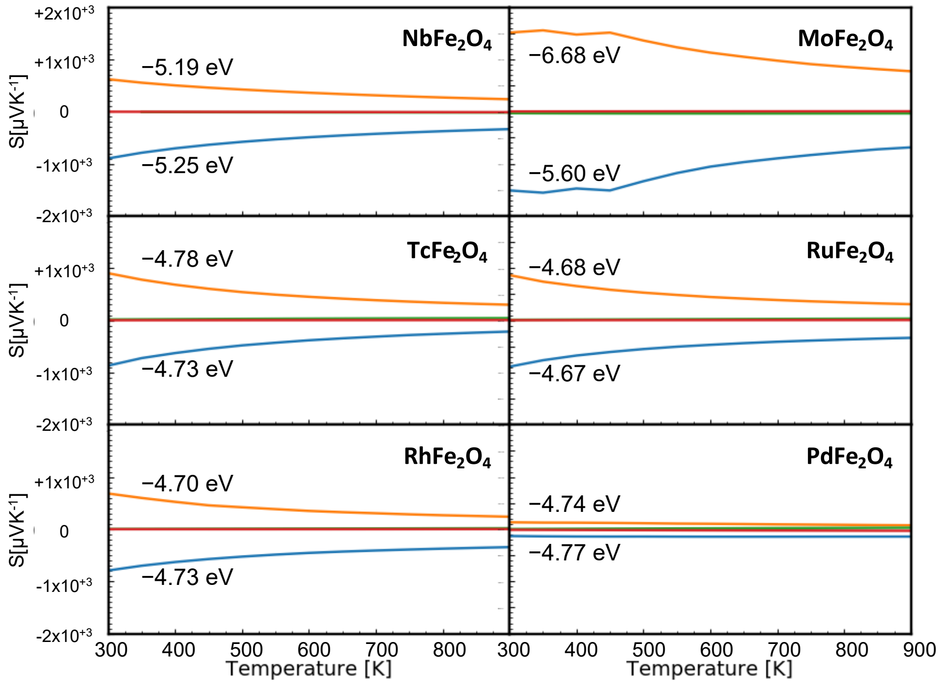


Figure S5. The Seebeck coefficient ($S$) for the 4d TM containing $TMFe_2O_4$ compounds as a function of temperature at different chemical potentials. The blue and orange lines indicate the chemical potentials for which $S$ was an absolute extreme.

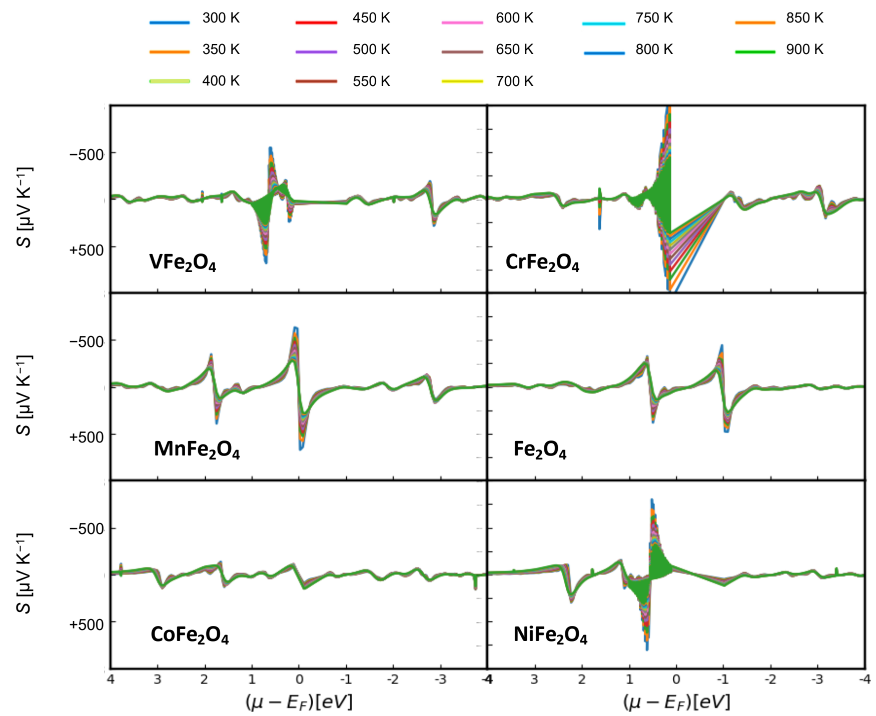


Figure S6. The Seebeck coefficient ($S$) for the 3d TM containing $TMFe_2O_4$ compounds as a function of the shift in the chemical potential ($\mu$) at different temperatures.

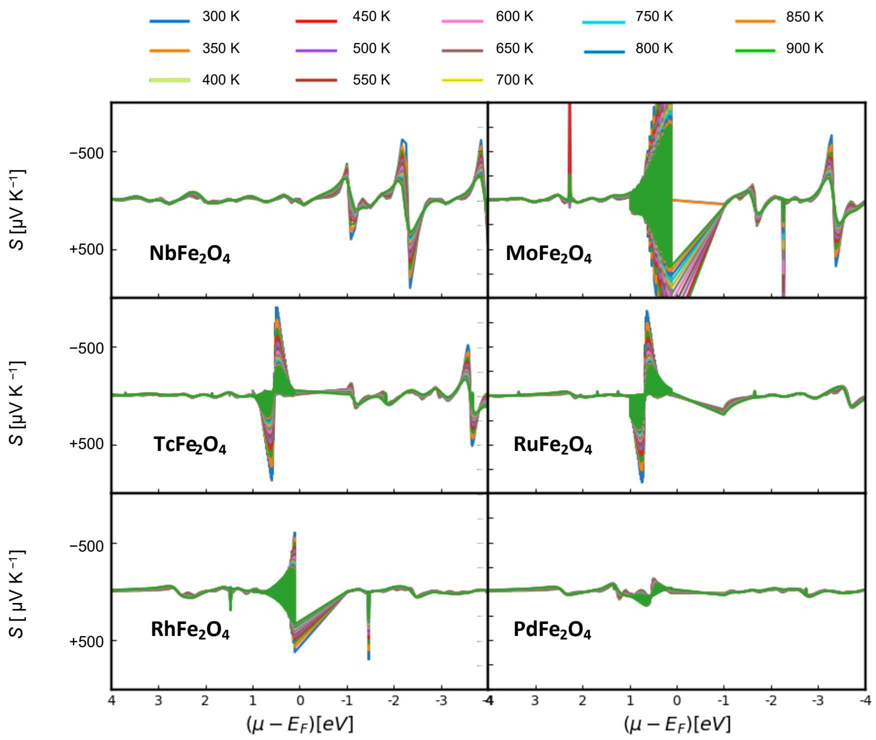


Figure S7. The Seebeck coefficient ($S$) for the 4d TM containing $TMFe_2O_4$ compounds as a function of the shift in the chemical potentia ($\mu$)l at different temperatures.

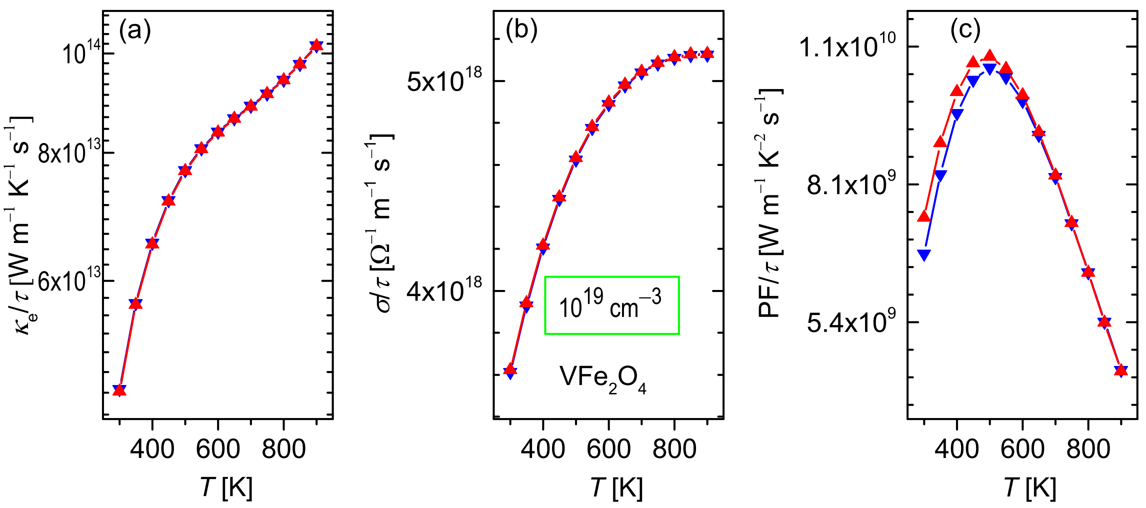


Figure S8. $\kappa_e$ / $\tau$ (a), $\sigma$ / $\tau$ (b), and PF/$\tau$ (c) for the half-metallic $VFe_2O_4$ compound. $\tau$, $\kappa_e$, $\sigma$, and PF stand for relaxation time, electronic contribution to the thermal conductivity, electric conductivity, and power factor, respectively. Here, due to the partially filled valence band, doping of the moderate $10^{19}$ carriers/cm$^3$ (blue symbols for electrons and red symbols for holes) does not affect the transport behavior significantly. Due to the half-metallic character, $\kappa_e$ / $\tau$ is $\sim$ 2 orders of magnitude larger than that of semiconducting $CrFe_2O_4$ of **Figure 6**.

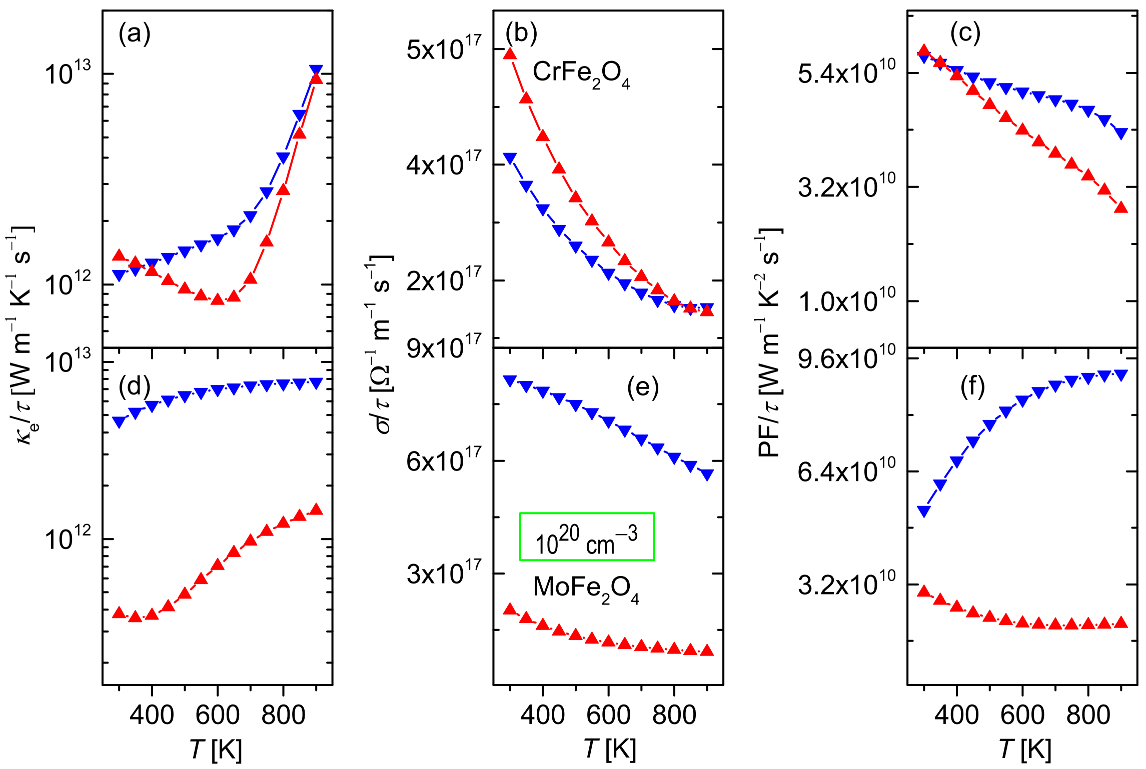


Figure S9. Upper row panels a, b, and c show the electronic contribution to the thermal conductivity per relaxation time ($\kappa_e$ / $\tau$), the electric conductivity per relaxation time ($\sigma$ / $\tau$), and the power factor per relaxation time (PF/$\tau$) for $CrFe_2O_4$, respectively. The lower row panels (d, e, and f) show the same quantities for $MoFe_2O_4$. Here, the carrier concentration is $10^{20}$ carriers/cm$^3$. Red and blue symbols indicate hole and electron doping, respectively. Given the higher carrier concentration, $\kappa_e/\tau$ and $\sigma/\tau$ are about an order of magnitude larger than the values reported for a doping level of $10^{19}$ carriers/cm$^3$ presented in **Figure 6**. Although, according to **Figure 4(b)**, the absolute $S$ value for $10^{20}$ carriers/cm$^3$ doped $CrFe_2O_4$ is smaller than that of $10^{19}$ carriers/cm$^3$ doped compound, the higher $\sigma/\tau$ results in slightly larger PF/$\tau$. Furthermore, since the decline in $S$ for $10^{20}$ carriers/cm$^3$ doped $CrFe_2O_4$ with rising $T$ does not occur as early as for that of $10^{19}$ carriers/cm$^3$ doped compound, the PF/$\tau$ does not drop with rising temperature as much.

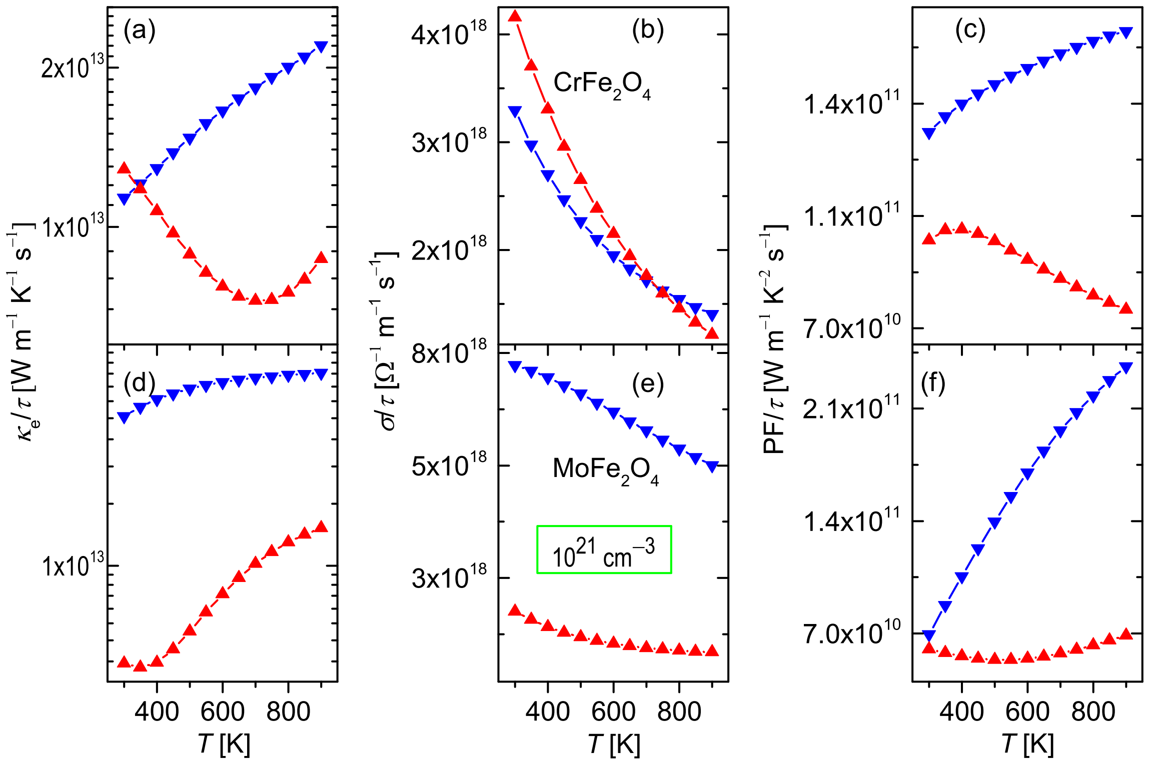


Figure S10. Upper row panels a, b, and c show the $\kappa_e\,/\,\tau$, $\sigma\,/\,\tau$, and PF/$\tau$ for $CrFe_2O_4$, respectively. The lower row panels (d, e, and f) show the same quantities for $MoFe_2O_4$. Here, the carrier concentration is $10^{21}$ carriers/cm$^3$. Red and blue symbols indicate hole and electron doping, respectively. Here, $\kappa_e\,/\,\tau$ and $\sigma\,/\,\tau$ are about an order of magnitude larger than the values reported for a doping level of $10^{20}$ carriers/cm$^3$ presented in Figure S9. Although, due to a compensating effect between $\sigma\,/\,\tau$ and $S$, PF/$\tau$ is still relatively high, the large $\kappa_e\,/\,\tau$ values, presented here, are detrimental to the thermoelectric application.

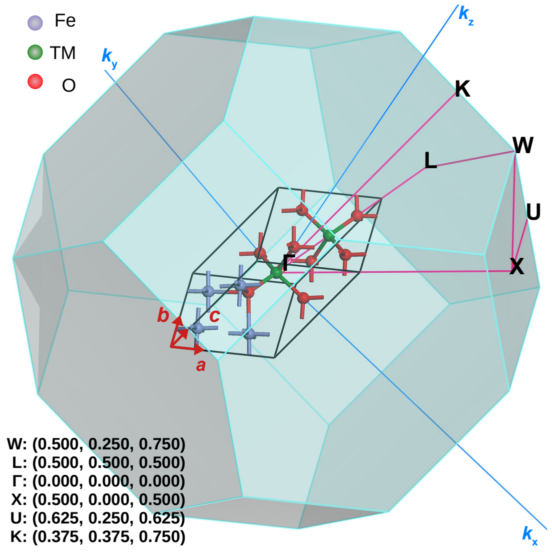


Figure S11. The reciprocal lattice and the high symmetry points and paths used for calculating the band structure of $CrFe_2O_4$ and $MoFe_2O_4$ in their trigonal representation, which is the primitive form of the face-centered cubic lattice structure (spinel structure). The paths were calculated using the `seekpath` package [S1].

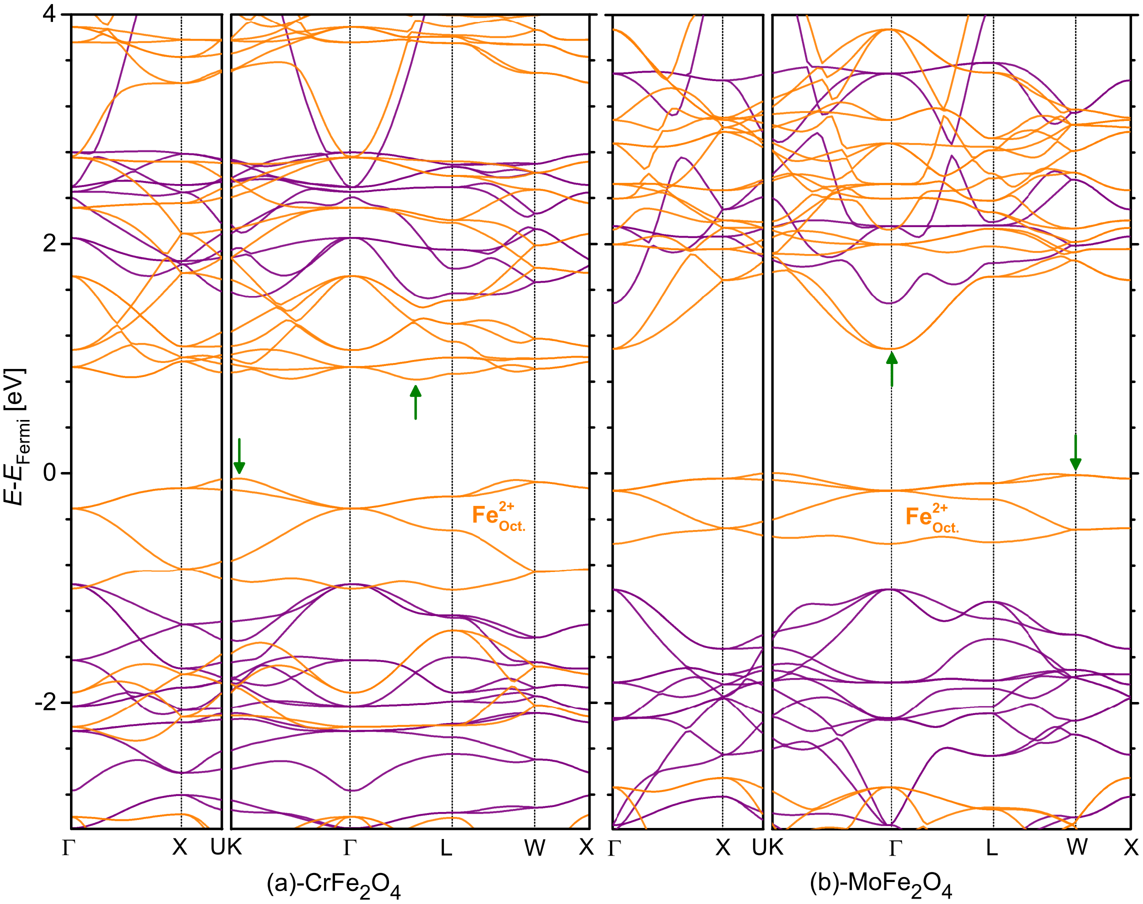


Figure S12. The band structure of the $CrFe_2O_4$ (a) and $MoFe_2O_4$ (b) compounds. Purple and orange lines represent spin-up and spin-down bands, respectively. Both compounds have indirect band gaps, as indicated by band extrema (marked with green arrows). The calculate electron effective mass $m_e^\star$ at the conduction band minimum and hole effective mass $m_h^\star$ at the valence band maximum shows that carriers in both compounds have anisotropic effective masses (see TABLE S2). The effective masses were calculated using the "effective mass calculator" code obtained from `https://github.com/afonari/emc`, which uses the finite difference method, without resorting to parabolic fitting around band extrema.

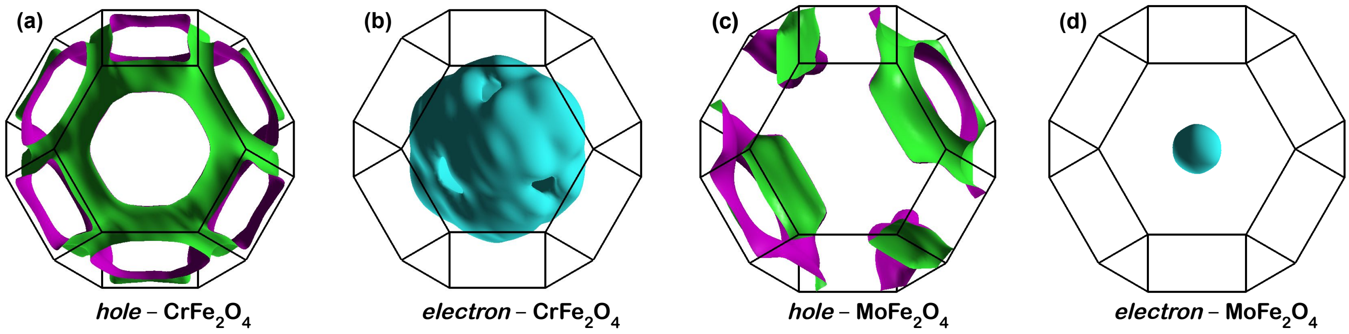


Figure S13. Fermi surfaces of $CrFe_2O_4$ (a, b), and $MoFe_2O_4$ (c, d), for the hole doping (a, c) at $\mu = -0.02$ eV, and electron doping (b, d) at $\mu = +0.02$ eV.

## SUPPLEMENTARY TABLES

TABLE S1. The approximate values of the Seebeck coefficient ($S$), the conductivity ($\sigma$), and the power factor (PF) of some high performing $p$- and $n$-type thermoelectric oxides. The values reported pertain to the temperatures for which PF was maximum—note that the list was not meant to be exhaustive. For comprehensive reviews, see the note.[a]

| Compound | Dopant | Concentration | $S$ [µV K$^{-1}$] | $\sigma$ [$\Omega^{-1}$ cm$^{-1}$] | PF [µW K$^{-2}$ m$^{-1}$] | $T$ [K] | Reference |
|---|---|---|---|---|---|---|---|
| $Ca_3Co_4O_9$ | Tb | 1.67% | 210 | 333 | 1500[b] | 800 | [S2] |
| $PbPdO_2$ | Li | 4% | 170 | 200 | 580[c] | 600 | [S3] |
| $Na_{0.8}CoO_2$ | Mg | 5% | 160 | 245 | 620[d] | 800 | [S4] |
| $CaMnO_3$ | Bi | 3% | −170 | 166 | 500[e] | 423 | [S5] |
| $SrTiO_3$ | Dy & La | 2% | −120 | 900 | 1300[f] | 550 | [S6] |
| $SrSnO_3$ | La | 1% | −130 | 70 | 120[g] | 1073 | [S7] |

[a] [S8–S12]
[b] With decreasing temperature, PF drops rapidly and monotonically to ∼ 150 µW K$^{-2}$ m$^{-1}$ at $T$ = 300 K.
[c] PF drops monotonically to ∼ 200 µW K$^{-2}$ m$^{-1}$ at $T$ = 300 K with decreasing $T$.
[d] PF drops substantially to ∼ 450 µW K$^{-2}$ m$^{-1}$ with decreasing temperature before rising back to ∼ 500 µW K$^{-2}$ m$^{-1}$ at $T$ = 300 K.
[e] PF drops to ∼ 400 µW K$^{-2}$ m$^{-1}$ for higher and lower temperatures.
[f] PF is only this high for a narrow temperature window. PF rapidly depreciates to ∼ 700 µW K$^{-2}$ m$^{-1}$ for $T$ = 300 K and $T$ = 1150 K.
[g] PF drops two orders of magnitude at $T$ = 400 K with decreasing temperature.

TABLE S2. The electron effective mass at the bottom of the conduction band ($m_e^\star$) and the hole effective mass at the top of the valence band ($m_h^\star$) along the $k_x$, $k_y$ and $k_z$ axes of the Brillouin zone (shown in Figure S11). $m_0$ is the electron mass at rest.

| compound | Electron/hole | $k_x$ | $k_y$ | $k_z$ | Harmonic mean |
|---|---|---|---|---|---|
| $CrFe_2O_4$ | $m_e^\star$ | $14.02m_0$ | $2.07m_0$ | $0.79m_0$ | $1.65m_0$ |
| | $m_h^\star$ | $0.16m_0$ | $0.30m_0$ | $2.09m_0$ | $0.30m_0$ |
| $MoFe_2O_4$ | $m_e^\star$ | $2.67m_0$ | $2.64m_0$ | $2.30m_0$ | $2.52m_0$ |
| | $m_h^\star$ | $0.33m_0$ | $0.33m_0$ | $1.43m_0$ | $0.45m_0$ |

* h.assadi.2008@ieee.org

[S1] Y. Hinuma, G. Pizzi, Y. Kumagai, F. Oba, and I. Tanaka, Comput. Mater. Sci. **128**, 140–184 (2017).
[S2] S. Saini, H. S. Yaddanapudi, K. Tian, Y. Yin, D. Magginetti, and A. Tiwari, Sci. Rep. **7**, 44621 (2017).
[S3] L. K. Lamontagne, G. Laurita, M. W. Gaultois, M. Knight, L. Ghadbeigi, T. D. Sparks, M. E. Gruner, R. Pentcheva, C. M. Brown, and R. Seshadri, Chem. Mater. **28**, 3367–3373 (2016).
[S4] P.-H. Tsai, M. H. N. Assadi, T. Zhang, C. Ulrich, T. T. Tan, R. Donelson, and S. Li, J. Phys. Chem. C **116**, 4324–4329 (2012).
[S5] R. Kabir, R. Tian, T. Zhang, R. Donelson, T. T. Tan, and S. Li, J. Alloys Compd. **628**, 347–351 (2015).
[S6] H. C. Wang, C. L. Wang, W. B. Su, J. Liu, Y. Sun, H. Peng, and L. M. Mei, J. Am. Ceram. Soc. **94**, 838–842 (2011).
[S7] M. Yasukawa, K. Ueda, S. Fujitsu, and H. Hosono, Ceram. Int. **43**, 9653–9657 (2017).
[S8] I. Terasaki, J. Appl. Phys. **110**, 053705 (2011).
[S9] T. M. Tritt, Annu. Rev. Mater. Res. **41**, 433–448 (2011).
[S10] S. Walia, S. Balendhran, H. Nili, S. Zhuiykov, G. Rosengarten, Q. H. Wang, M. Bhaskaran, S. Sriram, M. S. Strano, and K. Kalantar-zadeh, Prog. Mater. Sci. **58**, 1443–1489 (2013).
[S11] A. Nag and V. Shubha, J. Electron. Mater. **43**, 962–977 (2014).
[S12] Y. Feng, X. Jiang, E. Ghafari, B. Kucukgok, C. Zhang, I. Ferguson, and N. Lu, Adv. Compos. Hybrid Mater. **1**, 114–126 (2018).
